# Supplementary material for: Do We Need the Largest LLMs for Every Clinical Decision?
Source: arXiv:2610.26937 source file (2026-10-17)
Supplement: Supplementary file 2 [file si_tables.tex]

\newcommand{\tableSdecdist}{%
Qwen2.5-72B & 41.2 & 58.8 & 42.8 & 57.2 & 45.0/37.4 & 46.2/39.4 \\
HuatuoGPT-o1-72B & 40.5 & 59.5 & 41.9 & 58.1 & 42.8/38.2 & 43.6/40.2 \\
Med42-70B & 62.1 & 37.9 & 62.5 & 37.5 & 83.4/40.9 & 84.2/40.8 \\
OpenBioLLM-70B & 91.1 & 8.9 & 93.2 & 6.8 & 99.4/82.8 & 100.0/86.5 \\
MMed-Llama-3.1-70B & 86.8 & 13.2 & 89.0 & 11.0 & 100.0/73.6 & 100.0/77.9 \\
Llama-3.3-70B & 57.5 & 42.5 & 67.2 & 32.8 & 83.4/31.7 & 92.2/42.1 \\
Llama-3-70B & 60.3 & 39.7 & 64.3 & 35.7 & 83.3/37.3 & 89.9/38.7 \\
Llama-3-8B & 66.0 & 34.0 & 70.4 & 29.6 & 98.0/34.0 & 98.6/42.2 \\
MMed-Llama-3-8B & 74.0 & 26.0 & 67.7 & 32.3 & 99.4/48.5 & 99.3/36.1 \\
Mistral-7B & 51.8 & 48.2 & 47.8 & 52.2 & 72.3/31.4 & 67.5/28.1 \\
BioMistral-7B & 94.3 & 5.7 & 99.5 & 0.5 & 100.0/88.6 & 100.0/99.0 \\
}
\newcommand{\tableSperconfig}{%
Qwen2.5-72B & 100.0\,[100.0,100.0] & 100.0\,[100.0,100.0] & 93.6\,[92.1,94.9] & 100.0\,[100.0,100.0] & 100.0\,[100.0,100.0] \\
HuatuoGPT-o1-72B & 100.0\,[100.0,100.0] & 100.0\,[100.0,100.0] & 91.0\,[89.5,92.6] & 100.0\,[100.0,100.0] & 100.0\,[100.0,100.0] \\
Med42-70B & 99.8\,[99.6,100.0] & 100.0\,[100.0,100.0] & 56.3\,[53.7,59.2] & 0.0\,[0.0,0.0] & 97.5\,[96.6,98.4] \\
OpenBioLLM-70B & 100.0\,[100.0,100.0] & 100.0\,[100.0,100.0] & 84.7\,[82.6,86.6] & 86.9\,[85.0,88.9] & 98.1\,[97.3,98.8] \\
MMed-Llama-3.1-70B & 100.0\,[100.0,100.0] & 93.6\,[92.2,95.0] & 72.1\,[69.6,74.4] & 74.6\,[72.1,77.1] & 96.9\,[95.9,97.8] \\
Llama-3.3-70B & 100.0\,[100.0,100.0] & 100.0\,[100.0,100.0] & 51.9\,[49.2,54.7] & 38.1\,[35.4,40.8] & 82.2\,[80.0,84.2] \\
Llama-3-70B & 100.0\,[100.0,100.0] & 98.2\,[97.4,98.9] & 53.8\,[51.2,56.6] & 0.0\,[0.0,0.0] & 93.0\,[91.6,94.6] \\
Llama-3-8B & 100.0\,[100.0,100.0] & 100.0\,[100.0,100.0] & 15.0\,[13.0,17.1] & 100.0\,[100.0,100.0] & 92.8\,[91.4,94.2] \\
MMed-Llama-3-8B & 100.0\,[100.0,100.0] & 98.2\,[97.4,99.0] & 0.0\,[0.0,0.0] & 89.0\,[87.4,90.8] & 84.2\,[82.1,86.2] \\
Mistral-7B & 100.0\,[100.0,100.0] & 100.0\,[100.0,100.0] & 66.6\,[63.9,69.1] & 100.0\,[100.0,100.0] & 83.8\,[81.8,85.9] \\
BioMistral-7B & 100.0\,[100.0,100.0] & 80.3\,[78.2,82.6] & 56.1\,[53.4,58.9] & 100.0\,[100.0,100.0] & 95.8\,[94.6,96.8] \\
}
\newcommand{\tableSaudit}{%
Qwen2.5-72B & 1250 & 26 & 0.00 & 3.5 & 100.0 [100.0, 100.0] \\
HuatuoGPT-o1-72B & 1250 & 33 & 0.00 & 4.2 & 100.0 [100.0, 100.0] \\
Med42-70B & 1224 & 35 & 3.06 & 4.5 & 97.5 [96.6, 98.4] \\
OpenBioLLM-70B & 1224 & 37 & 0.31 & 4.7 & 98.1 [97.3, 98.8] \\
MMed-Llama-3.1-70B & 1223 & 29 & 0.12 & 3.9 & 96.9 [95.9, 97.8] \\
Llama-3.3-70B & 1048 & 32 & 8.25 & 4.9 & 82.2 [80.0, 84.2] \\
Llama-3-70B & 1151 & 34 & 3.50 & 4.7 & 93.0 [91.6, 94.6] \\
Llama-3-8B & 1149 & 30 & 1.12 & 4.3 & 92.8 [91.4, 94.2] \\
MMed-Llama-3-8B & 1046 & 30 & 0.61 & 4.7 & 84.2 [82.1, 86.2] \\
Mistral-7B & 1074 & 25 & 0.12 & 4.0 & 83.8 [81.8, 85.9] \\
BioMistral-7B & 1206 & 32 & 0.38 & 4.3 & 95.8 [94.6, 96.8] \\
}
\newcommand{\tableSmond}{%
Qwen2.5-72B & 517 & 11 & 0.34 & 97.4 & 4.9 & 722 & 6 & 0.12 & 100.0 & 2.5 \\
HuatuoGPT-o1-72B & 480 & 10 & 0.54 & 92.7 & 5.0 & 738 & 8 & 0.12 & 100.0 & 2.8 \\
Med42-70B & 762 & 18 & 3.71 & 97.7 & 4.6 & 433 & 4 & 10.78 & 88.2 & 3.4 \\
OpenBioLLM-70B & 1140 & 29 & 0.38 & 98.7 & 4.3 & 0 & 0 & $\infty$ & \emph{esc} & -- \\
MMed-Llama-3.1-70B & 1078 & 21 & 0.12 & 96.5 & 3.6 & 0 & 0 & $\infty$ & \emph{esc} & -- \\
Llama-3.3-70B & 612 & 13 & 10.62 & 72.3 & 4.6 & 420 & 0 & 0.25 & 100.0 & 1.6 \\
Llama-3-70B & 677 & 17 & 5.75 & 85.9 & 5.0 & 426 & 7 & 3.25 & 92.3 & 4.5 \\
Llama-3-8B & 775 & 20 & 1.62 & 89.6 & 4.9 & 370 & 3 & 0.62 & 94.8 & 3.5 \\
MMed-Llama-3-8B & 832 & 9 & 0.00 & 100.0 & 2.7 & 162 & 0 & 1.42 & 35.1 & 4.2 \\
Mistral-7B & 528 & 5 & 0.06 & 89.4 & 3.1 & 554 & 6 & 0.19 & 80.6 & 3.2 \\
BioMistral-7B & 1205 & 32 & 0.38 & 96.3 & 4.4 & 0 & 0 & $\infty$ & \emph{esc} & -- \\
}
\newcommand{\tableSclassres}{%
Qwen2.5-72B & 528 & 722 & 1.30 & 0.95 & 1.0 & certified \\
HuatuoGPT-o1-72B & 512 & 738 & 1.34 & 0.93 & 1.1 & certified \\
Med42-70B & 778 & 472 & 0.88 & 1.45 & 1.7 & certified \\
OpenBioLLM-70B & 1159 & 91 & 0.59 & 7.31 & 13.7 & \emph{resolution-limited} \\
MMed-Llama-3.1-70B & 1105 & 145 & 0.62 & 4.65 & 8.4 & \emph{risk-limited} \\
Llama-3.3-70B & 830 & 420 & 0.83 & 1.63 & 1.6 & certified \\
Llama-3-70B & 787 & 463 & 0.87 & 1.48 & 1.8 & certified \\
Llama-3-8B & 857 & 393 & 0.80 & 1.74 & 2.0 & certified \\
MMed-Llama-3-8B & 832 & 418 & 0.83 & 1.64 & 4.2 & certified \\
Mistral-7B & 590 & 660 & 1.16 & 1.04 & 1.4 & certified \\
BioMistral-7B & 1246 & 4 & 0.55 & 82.22 & 82.2 & \emph{resolution-limited} \\
}
\newcommand{\tableSgrid}{%
25 & 25.0 & 29.4 & 38.4 & 25.0 & 25.0 & 38.4 \\
50 & 25.0 & 28.2 & 38.4 & 25.0 & 25.0 & 38.4 \\
100 & 25.0 & 28.2 & 39.1 & 25.0 & 25.0 & 39.1 \\
200 & 25.0 & 28.2 & 39.1 & 25.0 & 25.0 & 39.1 \\
}
\newcommand{\tableSsplit}{%
Qwen2.5-72B & 25.0 & 25.0--25.0 & 25.0 & 25.0 \\
HuatuoGPT-o1-72B & 25.0 & 25.0--25.0 & 25.0 & 25.8 \\
Med42-70B & 27.8 & 26.8--28.3 & 25.0 & 29.3 \\
OpenBioLLM-70B & 27.2 & 26.6--27.6 & 25.7 & 27.9 \\
MMed-Llama-3.1-70B & 26.7 & 25.0--26.9 & 25.0 & 27.3 \\
Llama-3.3-70B & 38.4 & 36.8--39.0 & 35.8 & 40.7 \\
Llama-3-70B & 33.2 & 31.9--34.4 & 30.0 & 35.7 \\
Llama-3-8B & 29.9 & 29.2--30.3 & 27.6 & 31.5 \\
MMed-Llama-3-8B & 36.8 & 35.9--37.8 & 34.2 & 39.0 \\
Mistral-7B & 36.7 & 36.2--37.0 & 34.9 & 43.5 \\
BioMistral-7B & 27.9 & 26.9--28.0 & 26.6 & 28.7 \\
}
\newcommand{\tableSconfidence}{%
Qwen2.5-72B & 25.0 & 25.0 & 25.0 & 25.8 & 26.2 & 26.2 \\
HuatuoGPT-o1-72B & 25.0 & 25.0 & 25.0 & 27.3 & 27.6 & 28.2 \\
Med42-70B & 26.9 & 26.9 & 26.9 & 29.4 & 29.4 & 30.6 \\
OpenBioLLM-70B & 26.4 & 26.4 & 27.6 & 30.6 & 30.6 & 30.6 \\
MMed-Llama-3.1-70B & 27.3 & 27.3 & 27.3 & 35.2 & 35.2 & 35.2 \\
Llama-3.3-70B & 38.4 & 39.5 & 39.5 & 39.1 & 39.1 & 41.1 \\
Llama-3-70B & 30.2 & 30.2 & 31.8 & 33.9 & 35.1 & 37.4 \\
Llama-3-8B & 30.4 & 30.4 & 30.4 & 31.7 & 31.7 & 32.8 \\
MMed-Llama-3-8B & 36.8 & 36.8 & 39.0 & 40.2 & 40.2 & 48.4 \\
Mistral-7B & 37.1 & 37.1 & 37.1 & 36.3 & 36.3 & 36.3 \\
BioMistral-7B & 28.2 & 28.2 & 28.2 & 28.2 & 28.2 & 28.2 \\
}
\newcommand{\tableSmondalpha}{%
Qwen2.5-72B & 59.2 & 45.6 & 25.8 & 1.1 & 25.0 & 0.0 \\
HuatuoGPT-o1-72B & 72.6 & 45.3 & 27.3 & 3.1 & 25.0 & 0.0 \\
Med42-70B & 100.0 & 100.0 & 29.4 & 5.8 & 25.3 & 0.4 \\
OpenBioLLM-70B & 40.2 & 20.3 & 30.6 & 7.4 & 29.7 & 6.2 \\
MMed-Llama-3.1-70B & 41.3 & 21.7 & 35.2 & 13.6 & 26.6 & 2.1 \\
Llama-3.3-70B & 100.0 & 100.0 & 39.1 & 18.8 & 33.5 & 11.3 \\
Llama-3-70B & 100.0 & 100.0 & 33.9 & 11.9 & 26.2 & 1.6 \\
Llama-3-8B & 100.0 & 100.0 & 31.7 & 9.0 & 25.8 & 1.0 \\
MMed-Llama-3-8B & 52.3 & 36.4 & 40.2 & 20.2 & 34.2 & 12.2 \\
Mistral-7B & 100.0 & 100.0 & 36.3 & 15.1 & 29.2 & 5.6 \\
BioMistral-7B & 40.5 & 20.7 & 28.2 & 4.3 & 25.5 & 0.6 \\
}
\newcommand{\tableSexact}{%
Qwen2.5-72B & 25.8 & 26.7 & +0.9 & NF4 & Yes \\
HuatuoGPT-o1-72B & 27.3 & 27.9 & +0.6 & NF4 & Yes \\
Med42-70B & 29.4 & 30.6 & +1.3 & NF4 & Yes \\
OpenBioLLM-70B & 30.6 & 31.5 & +1.0 & NF4 & Yes \\
MMed-Llama-3.1-70B & 35.2 & 35.2 & +0.0 & NF4 & Yes \\
Llama-3.3-70B & 39.1 & 41.4 & +2.3 & NF4 & Yes \\
Llama-3-70B & 33.9 & 40.2 & +6.3 & NF4 & Yes \\
Llama-3-8B & 31.7 & 33.5 & +1.7 & NF4 & Yes \\
MMed-Llama-3-8B & 40.2 & 48.4 & +8.2 & NF4 & Yes \\
Mistral-7B & 36.3 & 36.3 & +0.0 & NF4 & Yes \\
BioMistral-7B & 28.2 & 28.2 & +0.0 & NF4 & Yes \\
}
\newcommand{\tableSexactaudit}{%
Qwen2.5-72B & 406 & 6 & 0.51 & 96.3 & 4.6 & 565 & 3 & 0.50 & 98.7 & 2.4 \\
HuatuoGPT-o1-72B & 378 & 5 & 0.54 & 92.7 & 4.5 & 576 & 4 & 0.38 & 98.6 & 2.7 \\
Med42-70B & 591 & 9 & 8.32 & 94.1 & 4.0 & 345 & 4 & 9.39 & 89.7 & 4.5 \\
OpenBioLLM-70B & 895 & 11 & 0.70 & 97.4 & 3.0 & 0 & 0 & $\infty$ & \emph{esc} & -- \\
MMed-Llama-3.1-70B & 861 & 16 & 0.05 & 96.5 & 3.9 & 0 & 0 & $\infty$ & \emph{esc} & -- \\
Llama-3.3-70B & 453 & 8 & 11.52 & 67.8 & 4.8 & 334 & 0 & 0.25 & 100.0 & 2.3 \\
Llama-3-70B & 488 & 9 & 8.12 & 77.0 & 4.8 & 308 & 2 & 6.20 & 84.8 & 3.8 \\
Llama-3-8B & 587 & 11 & 1.90 & 86.4 & 4.5 & 299 & 2 & 0.52 & 94.8 & 4.0 \\
MMed-Llama-3-8B & 660 & 6 & 0.02 & 100.0 & 2.9 & 0 & 0 & $\infty$ & \emph{esc} & -- \\
Mistral-7B & 424 & 3 & 0.05 & 89.4 & 3.2 & 445 & 4 & 0.18 & 80.6 & 3.5 \\
BioMistral-7B & 961 & 25 & 0.38 & 96.3 & 4.7 & 0 & 0 & $\infty$ & \emph{esc} & -- \\
}
\newcommand{\tableScalsize}{%
250 & 25.4 & 31.1 & 49.5 \\
500 & 25.0 & 27.9 & 44.5 \\
750 & 25.0 & 28.0 & 40.9 \\
1000 & 25.0 & 28.2 & 40.3 \\
1250 & 25.0 & 28.2 & 38.4 \\
}
\newcommand{\tableStaskwise}{%
RTN-8 & 100.0 & 1.1 & 100.0 & 1.4 \\
RTN-6 & 99.7 & 2.0 & 94.7 & 2.6 \\
RTN-4 & 60.0 & 1.9 & 56.5 & 3.7 \\
INT8 & 74.5 & 1.3 & 68.7 & 3.0 \\
NF4 & 94.6 & 2.3 & 91.5 & 3.8 \\
}
\newcommand{\tableSner}{%
\multicolumn{7}{l}{\textit{\textbf{BC5CDR-Disease}}}\\
Qwen2.5-72B & 0.720 & 0.720 & 0.735 & 0.669 & 0.713 & 0.956/0.568 \\
HuatuoGPT-o1-72B & 0.573 & 0.585 & 0.645 & 0.615 & 0.467 & 0.947/0.310 \\
Med42-70B & 0.852 & 0.853 & 0.852 & 0.694 & 0.829 & 0.895/0.773 \\
OpenBioLLM-70B & 0.705 & 0.705 & 0.710 & 0.684 & 0.573 & 0.925/0.415 \\
MMed-Llama-3.1-70B & 0.469 & 0.475 & 0.506 & 0.306 & 0.547 & 0.624/0.487 \\
Llama-3.3-70B & 0.866 & 0.876 & 0.881 & 0.849 & 0.862 & 0.948/0.791 \\
Llama-3-70B & 0.825 & 0.821 & 0.817 & 0.814 & 0.850 & 0.951/0.768 \\
Llama-3-8B & 0.641 & 0.642 & 0.659 & 0.718 & 0.611 & 0.938/0.454 \\
MMed-Llama-3-8B & 0.453 & 0.469 & 0.447 & 0.436 & 0.419 & 0.397/0.443 \\
Mistral-7B & 0.585 & 0.589 & 0.600 & 0.603 & 0.623 & 0.769/0.524 \\
BioMistral-7B & 0.384 & 0.389 & 0.400 & 0.440 & 0.405 & 0.506/0.338 \\
\midrule
\multicolumn{7}{l}{\textit{\textbf{NCBI-Disease}}}\\
Qwen2.5-72B & 0.747 & 0.749 & 0.752 & 0.742 & 0.747 & 0.951/0.615 \\
HuatuoGPT-o1-72B & 0.664 & 0.657 & 0.674 & 0.668 & 0.600 & 0.969/0.435 \\
Med42-70B & 0.719 & 0.721 & 0.704 & 0.649 & 0.608 & 0.894/0.460 \\
OpenBioLLM-70B & 0.583 & 0.583 & 0.578 & 0.502 & 0.546 & 0.931/0.386 \\
MMed-Llama-3.1-70B & 0.273 & 0.238 & 0.252 & 0.075 & 0.364 & 0.530/0.277 \\
Llama-3.3-70B & 0.712 & 0.718 & 0.725 & 0.755 & 0.691 & 0.951/0.543 \\
Llama-3-70B & 0.680 & 0.676 & 0.672 & 0.688 & 0.675 & 0.939/0.527 \\
Llama-3-8B & 0.667 & 0.676 & 0.668 & 0.663 & 0.690 & 0.949/0.542 \\
MMed-Llama-3-8B & 0.424 & 0.405 & 0.382 & 0.399 & 0.510 & 0.655/0.418 \\
Mistral-7B & 0.472 & 0.475 & 0.497 & 0.497 & 0.467 & 0.863/0.320 \\
BioMistral-7B & 0.432 & 0.461 & 0.488 & 0.414 & 0.479 & 0.659/0.376 \\
}
\newcommand{\tableSprev}{%
\textbf{Maximum over models} & marginal & 9.5 & 8.0 & 6.6 & 5.7 & 6.3 & 6.6 \\
 & Mondrian & 2.7 & 2.8 & 3.1 & 3.5 & 3.8 & 3.9 \\
\textbf{Mean over models} & marginal & 3.7 & 3.5 & 3.4 & 3.3 & 3.1 & 3.1 \\
 & Mondrian & 1.8 & 1.8 & 1.9 & 2.0 & 2.0 & 2.1 \\
\midrule
Qwen2.5-72B & marginal & 2.6 & 3.2 & 3.7 & 4.2 & 4.7 & 4.9 \\
 & Mondrian & 1.8 & 2.1 & 2.4 & 2.7 & 3.1 & 3.2 \\
HuatuoGPT-o1-72B & marginal & 3.1 & 3.4 & 3.8 & 4.1 & 4.5 & 4.7 \\
 & Mondrian & 1.5 & 1.6 & 1.6 & 1.7 & 1.8 & 1.8 \\
Med42-70B & marginal & 4.0 & 3.8 & 3.7 & 3.5 & 3.4 & 3.3 \\
 & Mondrian & 2.7 & 2.7 & 2.7 & 2.8 & 2.8 & 2.9 \\
OpenBioLLM-70B & marginal & 9.5 & 8.0 & 6.6 & 5.2 & 3.8 & 3.1 \\
 & Mondrian & 2.4 & 2.4 & 2.4 & 2.4 & 2.4 & 2.4 \\
MMed-Llama-3.1-70B & marginal & 3.7 & 3.2 & 2.6 & 2.1 & 1.6 & 1.4 \\
 & Mondrian & 1.1 & 1.1 & 1.1 & 1.1 & 1.1 & 1.1 \\
Llama-3.3-70B & marginal & 2.0 & 2.4 & 2.8 & 3.2 & 3.6 & 3.8 \\
 & Mondrian & 1.0 & 1.1 & 1.3 & 1.5 & 1.7 & 1.8 \\
Llama-3-70B & marginal & 3.9 & 4.5 & 5.1 & 5.7 & 6.3 & 6.6 \\
 & Mondrian & 2.5 & 2.8 & 3.1 & 3.5 & 3.8 & 3.9 \\
Llama-3-8B & marginal & 2.0 & 2.2 & 2.4 & 2.6 & 2.8 & 2.9 \\
 & Mondrian & 1.3 & 1.3 & 1.4 & 1.5 & 1.5 & 1.6 \\
MMed-Llama-3-8B & marginal & 4.6 & 3.7 & 2.7 & 1.8 & 1.0 & 0.5 \\
 & Mondrian & 1.9 & 1.8 & 1.7 & 1.6 & 1.6 & 1.5 \\
Mistral-7B & marginal & 3.2 & 2.6 & 2.0 & 1.4 & 0.7 & 0.3 \\
 & Mondrian & 1.0 & 0.9 & 0.7 & 0.6 & 0.5 & 0.4 \\
BioMistral-7B & marginal & 2.0 & 2.1 & 2.1 & 2.2 & 2.2 & 2.2 \\
 & Mondrian & 2.3 & 2.3 & 2.3 & 2.3 & 2.3 & 2.3 \\
}
